# Supplementary material for: Improving Lexically Constrained Neural Machine Translation with Source-Conditioned Masked Span Prediction
Source: arXiv:2105.05498 source file (2021-08-12)
Supplement: Supplementary file 1 [file appendix.tex]

% \appendix 

% \section{Preprocessing and Training}

% \subsection{Preprocessing} 
% \label{appendix:preprocessing}

% For De→En, we applied the Moses tokenization scripts and a joint source-target byte pair encoding (BPE) \cite{sennrich-etal-2016-neural} with 20,000 split operations. For En→Ko, English was tokenized using spaCy\footnote{\url{https://spacy.io/}} and Korean using KoNLPy's MeCab-ko\footnote{\url{https://konlpy.org/en/latest/}} \cite{park2014konlpy}, followed by BPE with 20,000 operations. We apply sentence filtering up to 80 tokens.

% \subsection{Training Setup} 
% \label{appendix:training_setup}

% We follow the base transformer architecture and fix the same hyperparamter configurations for all baselines. For the exact implementation of each baseline, we followed the authors' official code on github (\textsc{Chen20}\footnote{\url{https://github.com/ghchen18/leca}} and \textsc{Susanto20}\footnote{\url{https://github.com/raymondhs/constrained-levt}}, respectively). For all experiments, we implement models using \textsc{fairseq}\footnote{\url{https://github.com/pytorch/fairseq}} \cite{ott2019fairseq} trained on Nvidia GeForce RTX 3090 GPUs.

% \subsection{Hyperparameter}
% \label{appendix:hyperparamter}

% Detailed hyperparameter settings of transformers used in baselines are reported below. Span masking and task coefficient apply to our proposed method.

% \begin{table}[h!]
% \centering
% % \scriptsize
% \begin{tabular}{c|c}
% \hline
% \multicolumn{2}{c}{Transformer} \\
% \hline
% Embedding dim. & 512 \\
% Transformer FFN dim. & 2048 \\
% Enc/Decoder layers & 6 \\
% Attention heads & 8 \\
% Share all embedding & True \\
% Dropout & 0.3 \\
% Label smoothing & 0.1 \\
% Optimizer & Adam \\
% Learning rate & 0.0005 \\
% Warmup updates & 4000 \\
% Maximum token per batch & 4096 \\
% Maximum token lengths & 80 \\
% % Validation updates & 50 \\
% % Patience & 100 \\
% \hline
% \multicolumn{2}{c}{Span Masking} \\
% \hline
% Span length & Geometric (p=0.2) \\
% Maximum span length. & 10 \\
% Minimum span length. & 1 \\
% Corruption ratio & 0.5 \\
% \hline
% \multicolumn{2}{c}{Task Coefficient} \\
% \hline
% Task coefficient (\gamma) & 0.5 \\
% \hline
% \end{tabular}
% \caption{Hyperparameter settings}
% \label{tab:hyperparam}
% \end{table} 



% \section{LSM}

% \label{appendix:lsm}
% \SetAlFnt{\small}
% \begin{algorithm}[h]
% \caption{LSM algorithm}
% \KwData{Generated sentence $\tilde{y}$, Terminologies y'}
% \KwResult{Score }

% \SetKwProg{makesublist}{Make$\_$sublist}{ }{}
%   \makesublist{(Terminology T) : }{
%   \STATE {consecutive\_sub\_string $css$ = [] \newline}
%   \STATE {tokens = T.split(" ") \newline}
%   \STATE {n = ngram(T) \newline}
%   \ForEach{step in range(1, n)}
%         {
%             \ForEach{i in range(0, n - step)}
%             {
%                 $css$.append( " ".join(tokens[i:i+step+1]) )
%             }
%         }
%     \Return $css$
% }

% \SetKwProg{getstat}{Get$\_$stat}{ }{}
%   \getstat{(Sentence S, Terminology T) : }{
%       \eIf{T in S}{
%       \Return ngram(S), T
%     }{
%     sub$\_$string$\_$list = Make$\_$sublist(T)
    
%     \ForEach { sub$\_$string $s_i$ in sub$\_$string$\_$list}
%         {
%         \If {$s_i$ in S}
%             {
%             \Return ngram($s_i$), sub$\_$string 
%             }
%             }
%     \Return 0, NULL 
%   }
% }


% \begin{algorithmic}[1]

% \FORALL{ y$\_i'$ in y'}{ 
% \STATE {reference$\_$n = ngram(y$\_i'$)}
% \STATE{matched$\_$n, $\_$ = get$\_$stat( $\tilde{y}$, y$\_i'$)} 
% }
% \STATE{Score += ( matched$\_$n / reference$\_$n ) }
% \ENDFOR
% \end{algorithmic}
% \end{algorithm}



% For instance, suppose we would like to calculate a partial matching score of \textit{``local public official''} given the generated terminology, \textit{``local public person''}. We first generate all possible sub-sequences of the reference terminology length $\geq$2, which are [\textit{local public, public official, local public official}]. Then, LSM summarizes the score by the longest sub n-gram matching divided by the total length of terminology tokens, which is 2/3 in this case. Since we found that uni-gram overlaps are too frequent and spurious to match what we intended, we disregard uni-gram overlaps. 


% % \subsection{Effect of mask ratio} 
% % \label{appendix:mask_ratio}

% % We analyze the effect of mask ratio of [0.25, 0.5, 0.75] on Law De→En data. The effect of masking ratio evaluated in BLEU is illustrated below:



% \section{Terminology-aware Data Split Algorithm}


% \label{appendix:data_split}
% \SetAlFnt{\small}
% \begin{algorithm}[h]
% \caption{Terminology-aware data split algorithm}
% \KwData{Dictionary $\mathbb{D}$, Corpus $\mathbb{C}$, TestSize \textit{R}}
% \KwResult{Sent=(Sent$_{train}$, Sent$_{valid}$, Sent$_{test}$) \newline
% Term=(Term$_{train}$, Term$_{valid}$, Term$_{test}$)}
% \begin{algorithmic}[1]
% \STATE Initialize terminologies $\mathbb{T}$ by n-gram in descending order from {$\mathbb{D}$}
% \STATE {\textit{N}} = dict()
% \STATE {\textit{P'}} = dict()

%   \FORALL{ (x, y) in $\mathbb{C}$}
%     \STATE {\textit{ngramlist}} = []
%     \STATE {\textit{P''}} = []
%     \FORALL{ (x', y') in {$\mathbb{T}$}}
%       \IF { y' in y and x' in x  }
%         \STATE { {\textit{ngramlist}} += ngram(y')  }
%         \STATE { y = y.replace(y', ``", 1) }
%         \STATE { {\textit{P''}} += (x', y')  }

%       \ENDIF 
%     \ENDFOR
    
%     \STATE {\textit{n}} = Max({\textit{ngramlist}})
%     \IF { n is not in {\textit{N}}.keys() }
%     \STATE { {\textit{N}}[{\textit{n}}] = [] }
%     \ENDIF
    
%     \STATE {\textit{N}}[{\textit{n}}] += (x, y)
%     \STATE {\textit{P'}}[y] = {\textit{P''}}
%   \ENDFOR

% \STATE {\textit{K}} = ngrams sorted in descending order in {keys of \textit{N}}
% \STATE Size = ( $|\textit{C}|$ - 2 * \textit{R}, \textit{R}, \textit{R} )

% \FORALL{{\textit{k}} in {\textit{K}}}
%     \STATE {$S_d$ , $S_u$ = DuplicateCheck($N$[$k$], {\textit{P'}})}
%     \STATE {Sent, Term += DuplicateSampling($S_d$, {\textit{P'}}, Size)}
%     \STATE {Sent, Term += UniqueSampling($S_u$, {\textit{P'}}, Size) }
% \ENDFOR

% \end{algorithmic}
% \label{algo:data_split}
% \end{algorithm}

% \begin{small}
% \noindent 
% Line 2 : Initialize a dictionary for storing sentence pairs by matched maximum terminology length \\
% Line 3 : Initialize a dictionary for storing matched terminologies for each target sentence \\
% Line 5 : Temporarily initialize to store the lengths of terminologies in a sentence \\
% Line 6 : Temporarily initialize a matched terminology list in a sentence \\
% Line 9 : ngram() returns the token length of a terminology \\
% Line 22 : For each Size=(TrainSize, ValidSize, TestSize), values decrease as sentences are distributed to each data split by DuplicateSampling() and UniqueSampling(). When a size reaches zero, the assignment process stops at the split. \\
% Line 24 : DuplicateCheck() distinguishes between duplicate sentences $S_d$ and unique sentences $S_u$ from $S$.  \\
% Line 25 : DuplicatingSampling() calculates the ratio to be distributed to train, valid, and test based on Size, and then returns duplicate sentences and phrases for each split.   \\
% Line 26 : UniqueSampling() evenly distributes sentences and phrases alternatively between train, valid, and test. \\
% \end{small}

% % In terminology-aware data split algorithm, first, it sorts terminology from long to short n-gram in dictionary. Then, 

% % First we sort the terminology from the dictionary from long n-gram to short n-gram. Then, from the long terminology, it matches each sentence of the corpus to find all the terminology belonging to each sentence.
% % After that, the entire sentences are sorted in descending order based on the longest n-gram terminology among the matched terminologies for each sentence.
% % The entire corpus sorted based on n-gram is divided into train, valid, and test, one by one in descending order. At this time, duplicate sentences may exist due to the nature of the data, and duplicate sentences are sequentially distributed through the duplicateSampling function according to the ratio of the train, valid, and test sizes to be divided. And, sentences that do not overlap are sequentially distributed to each data set through the uniquesampling function.


% %While distributing data through DuplicateSampling and UniqueSampling, the size of each element of the Size variable is reduced, and the sizes of sentences allocated to the train, valid, and test datasets are checked. Finally, in the algorithm, phrase variable means 

% % 처음에 우리는 사전으로부터 길이가 긴 n-gram부터 짧은 n-gram 순서로 terminology를 정렬한다. 그리고 나서 길이가 긴 terminology부터 코퍼스의 각 문장들과 매칭시켜 각 문장에 속하는 terminology를 모두 구한다.
% % 이후 각 문장마다 매칭된 terminology 중 가장 긴 n-gram의 terminology를 기준으로 전체 문장을 내림차순으로 정렬한다. 
% % n-gram을 바탕으로 정렬된 전체 코퍼스를 내림차순으로 하나씩 번갈아가며 train, valid, test로 분할한다. 이 때, 데이터 특성상 중복된 문장들이 존재할 수 있는 데, 나누려고 하는 train, valid, test 크기 비율에 따라 duplicateSampling 함수를 통해 중복된 문장들을 순차적으로 분배해준다. 그리고, 중복되지 않는 문장들은 uniquesampling 함수를 통해 순차적으로 각 데이터셋에 분배해준다.
% % DuplicateSampling과 uniquesampling을 통해 데이터를 분배해가며, Size 변수의 각 원소의 크기를 줄여가며, train, valid, test dataset에 할당받는 문장의 크기를 확인한다. 그리고 여기서 phrase 변수는 각 데이터 코퍼스에 매칭되는 terminology를 뜻한다.

% \clearpage


% \section{Qualitative Examples}
% \label{appendix:qual_ex}

% \begin{table*}
% \centering
% \begin{tabular}{l|l}
% \multicolumn{2}{l}{\textit{Law Ko-En}}       \\ 
% \hline
% Source      &                                \\
% model1      &                                \\
% model2      &                                \\
% model3      &                                \\
% model4      &                                \\
% model5      &                                \\
% Reference   &                                \\
% Terminology &                                \\ 
% \hline
% \multicolumn{2}{l}{\textit{Acquis De-En}}    \\ 
% \hline
% Source      &                                \\
% model1      &                                \\
% model2      &                                \\
% model3      &                                \\
% model4      &                                \\
% model5      &                                \\
% Reference   &                                \\
% Terminology &                                \\ 
% \hline
% \multicolumn{2}{l}{\textit{Emea De-En}}      \\ 
% \hline
% Source      &                                \\
% model1      &                                \\
% model2      &                                \\
% model3      &                                \\
% model4      &                                \\
% model5      &                                \\
% Reference   &                                \\
% Terminology &                                \\
% \hline
% \end{tabular}
% \caption{Examples of our model and baselines}
% \end{table*}

% \clearpage

% \begin{table*}
% \centering
% \renewcommand{\arraystretch}{1.5}
% \resizebox{\textwidth}{!}{\begin{tabular}{|l|l|l|l|l|l|l|l|l|l|} 
% \hline
% \multicolumn{10}{|c|}{\textbf{DINU dataset }}   \\ 
% \hline
% \multicolumn{10}{|c|}{\textbf{Iate-414 }}   \\ 
% \hline
% \textbf{Number of sentences} & 414  & \textbf{Number of terminology} & 452 (217) & \textbf{Average term per sentence} & 1.09 & \textbf{Average n-gram} & 1.15 & \textbf{Short(\textless{}=2) n-gram ratio} & 98.45\%  \\ 
% \hline
% \textbf{The 10 most frequent terminology} & \multicolumn{9}{l|}{'gold', 'CDU', 'bridge', 'China', 'Syria', 'night', 'campaign', 'generation', 'month'. 'Iraq'}   \\ 
% \hline
% \multicolumn{10}{|c|}{\textbf{Iate-581}} \\ 
% \hline
% \textbf{Number of sentences} & 581  & \textbf{Number of terminology} & 659 (269)    & \textbf{Average term per sentence} & 1.13 & \textbf{Average n-gram} & 1.13 & \textbf{Short(\textless{}=2) n-gram~ratio} & 98.63\%  \\ 
% \hline
% \textbf{The 10 most frequent terminology} & \multicolumn{9}{l|}{'gold', 'doping', 'CDU', 'sport', 'US', 'bridge', 'Syria', 'campaign', 'China', 'night'} \\ 
% \hline
% \multicolumn{10}{|c|}{\textbf{Wikt-727}} \\ 
% \hline
% \textbf{Number of sentences} & 727  & \textbf{Number of terminology} & 884 (333) & \textbf{Average term per sentence} & 1.21 & \textbf{Average n-gram} & 1.11 & \textbf{Short(\textless{}=2) n-gram~ratio} & 98.30\%  \\ 
% \hline
% \textbf{The 10 most frequent terminology} & \multicolumn{9}{l|}{'percent', 'police', 'Thursday', 'Putin', 'five', 'September', 'Venus', 'later', 'Tuesday', 'less'}  \\ 
% \hline
% \multicolumn{10}{|c|}{\textbf{Wikt-975}} \\ 
% \hline
% \textbf{Number of sentences} & 975  & \textbf{Number of terminology} & 1248 (451)   & \textbf{Average term per sentence} & 1.28 & \textbf{Average n-gram} & 1.10 & \textbf{Short(\textless{}=2) n-gram~ratio} & 98.80\%  \\ 
% \hline
% \textbf{The 10 most frequent terminology} & \multicolumn{9}{l|}{'percent', 'police', 'Thursday', 'Putin', 'old', 'September', 'five', 'swimmer', 'later', 'Venus'}  \\ 
% \hline
% \multicolumn{10}{|c|}{\textbf{Our dataset}} \\ 
% \hline
% \multicolumn{10}{|c|}{\textbf{Law (De -\textgreater{} En)}} \\ 
% \hline
% \textbf{Number of sentences} & 3000 & \textbf{Number of terminology} & 14018 (2521) & \textbf{Average term per sentence} & 4.67 & \textbf{Average n-gram} & 2.65 & \textbf{Short(\textless{}=2) n-gram~ratio} & 82.66\%  \\ 
% \hline
% \textbf{The 10 most frequent terminology} & \multicolumn{9}{l|}{'Council', 'Regulation', 'Commission', 'Union', 'Treaty', 'Official Journal', 'Member State', 'proposal', 'on a proposal from the Commission', 'market'} \\ 
% \hline
% \multicolumn{10}{|c|}{\textbf{Medical (De -\textgreater{} En)}}  \\ 
% \hline
% \textbf{Number of sentences} & 3000 & \textbf{Number of terminology} & 13319 (1879) & \textbf{Average term per sentence} & 4.43 & \textbf{Average n-gram} & 1.68 & \textbf{Short(\textless{}=2) n-gram~ratio} & 74.67\%  \\ 
% \hline
% \textbf{The 10 most frequent terminology} & \multicolumn{9}{l|}{'injection', 'water', 'water for injection', 'patient', 'infusion', 'solution for infusion', 'sodium', 'distribution', 'volume of distribution', 'treatment'} \\ 
% \hline
% \multicolumn{10}{|c|}{\textbf{Law (Ko -\textgreater{} En)}} \\ 
% \hline
% \textbf{Number of sentences} & 3000 & \textbf{Number of terminology} & 14159 (1287) & \textbf{Average term per sentence} & 4.71 & \textbf{Average n-gram} & 1.53 & \textbf{Short(\textless{}=2) n-gram~ratio} & 78.26\%  \\ 
% \hline
% \textbf{The 10 most frequent terminology} & \multicolumn{9}{l|}{'si', 'official', 'public official', 'member', 'term of office', 'gu', 'education', 'period', 'term', 'management'} \\
% \hline
% \end{tabular}}
% \end{table*}

% \section{Detailed terminology generation result on Acquis}
% \begin{table*}
% % \centering
% % % \scriptsize
% % \begin{tabular}{lcccccl}\toprule
% % & \multicolumn{3}{c}{Law} & \multicolumn{3}{c}{Medical}
% % \\\cmidrule(lr){2-4}\cmidrule(lr){5-7}
% %           & en-de  & de-en & en-fr    & en-de  & de-en & en-fr \\\midrule
% % \textsc{FW}        & 51.93 & 59.06 & 54.04 & 43.69 & 62.10 & 70.38 \\
% % \textsc{biTM}      & 50.95 & 61.89 & 55.17 & 48.41 & 64.71 & 68.27 \\
% % \textsc{NCM(biTM+LM)}   & 53.12 & 62.11 & 57.34 & 45.32 & 64.22 & 72.52 \\
% % \textsc{BERT-NMT}  & 46.50 & 59.01 & 53.07 & 41.55 & 59.46 & 65.05 \\
% % \textsc{LegalBERT} & 47.11 & 59.72 & 52.64 & - & - & - \\
% % \textsc{PubmedBERT} & - & - & - & 41.40 & 59.50 & 65.68 \\
% % \textsc{Language Prior}   & 49.51 & 59.04 & 54.12 & 43.10 & 62.12 & 70.58 \\
% % \textsc{RC(biTM+RC)}   & 52.10 & 60.01 & 55.01 & 48.87 & 64.28 & 70.89 \\\hline
% % \textsc{New model} & 54.51 & 63.18 & 57.68 & 50.29 & 66.64 & 73.24 \\\bottomrule
% % \end{tabular}
% \caption{Detailed result \label{table1}}
% \end{table*}






% %%%%%%%%%%%%%%%%%%%%%%%%%%%%%%%%%%%%%%%%%%%%%%%%%%%%%%%%%%%%%%%%%% 
% %%%%%%%%%%%%%%%%%%%%%%%%%%%%%%%%%%%%%%%%%%%%%%%%%%%%%%%%%%%%%%%%%%
% %%%%%%%%%%%%%%%%%%%%%%%%%%%%%%%%%%%%%%%%%%%%%%%%%%%%%%%%%%%%%%%%%%
% %%%%%%%%%%%%%%%%%%%%%%%%%%%%%%%%%%%%%%%%%%%%%%%%%%%%%%%%%%%%%%%%%%

% \clearpage

% \section{Reproducibility Checklist}

% Before you submit, please make sure that the following reproducibility checklist is filled.
% For all reported experimental results:
% \begin{itemize}
%     \item {A clear description of the mathematical setting, algorithm, and/or model (O)}

%     \item {Submission of a zip file containing source code, with specification of all dependencies, including external libraries, or a link to such resources (while still anonymized) (TODO)}

%     \item {Description of computing infrastructure used (O)}

%     \item {Average runtime for each approach (X)}

%     \item {Number of parameters in each model (O)}

%     \item {Corresponding validation performance for each reported test result (X)}

%     \item {Explanation of evaluation metrics used, with links to code (O)}

% \end{itemize}

% For all experiments with hyperparameter search:
% \begin{itemize}

%     \item {Bounds for each hyperparameter (O)}

%     \item {Hyperparameter configurations for best-performing models (O)}
    
%     \item {Number of hyperparameter search trials (X)}

%     \item {The method of choosing hyperparameter values (e.g., uniform sampling, manual tuning, etc.) and the criterion used to select among them (e.g., accuracy) (O)}

%     \item {Expected validation performance, or the mean and variance as a function of the number of hyperparameter trials (X)}
    
% \end{itemize}    


% For all datasets used:
% \begin{itemize}
%     \item {Relevant statistics such as number of examples (TODO)}
    
%     \item {Details of train/validation/test splits (O)}

%     \item {Explanation of any data that were excluded, and all pre-processing steps (O)}
    
%     \item {A link to a downloadable version of the data (O)}

%     \item {For new data collected, a complete description of the data collection process, such as instructions to annotators and methods for quality control (O)}

% \end{itemize}
